# Supplementary material for: The Configurable SAT Solver Challenge (CSSC)
Source: arXiv:1505.01221 source file (2016-08-02)
Supplement: Supplementary file 1 [file appendix.tex]

\clearpage
\note{The following appendices just give more results, we will drop them for submission.}

\section{Tables for each Track}

\begin{table}[th]
\sffamily\small\centering
\setlength\tabcolsep{0.3em}
\begin{tabular}{l | ccccc | ccccc}
\toprule[1pt]
 & \multicolumn{5}{c|}{Training} & \multicolumn{5}{c}{Test}\\
 & \smac{}-d & \smac{}-c & \pils{} & \gga{}-d & \gga{}-c & \smac{}-d & \smac{}-c & \pils{} & \gga{}-d & \gga{}-c  \\
\midrule
 \multicolumn{11}{c}{CSSC-K3-300s-2day}\\
\midrule
\clasp & $2.7$ & $2.8$ & $2.5$ & -- & -- & $2.5$ & $3.0$ & $2.4$ & -- & --\\
\dccsat & $4.8$ & $4.9$ & $4.8$ & -- & $4.9$ & $4.9$ & $4.9$ & $4.9$ & -- & $5.0$\\
\riss & $3.3$ & $3.0$ & $2.9$ & $0.2$ & $0.3$ & $1.3$ & $2.2$ & $1.9$ & $0.2$ & $0.4$\\
\minisathack & $4.4$ & $4.0$ & $4.4$ & $2.2$ & $0.9$ & $5.2$ & $5.2$ & $5.3$ & $2.8$ & $1.7$\\
\sparrow & $11.6$ & $11.2$ & $7.9$ & -- & -- & $5.4$ & $8.3$ & $6.7$ & -- & --\\
\midrule
 \multicolumn{11}{c}{CSSC-3cnf-v350-300s-2day}\\
\midrule
\minisathack & $7.2$ & $7.1$ & $10.2$ & -- & $0.8$ & $9.8$ & $6.8$ & $6.9$ & -- & $1.1$\\
\dccsat & $4.4$ & $4.4$ & $4.4$ & $4.3$ & $4.3$ & $4.9$ & $4.8$ & $4.9$ & $4.8$ & $4.8$\\
\riss & $3.6$ & $4.0$ & $3.4$ & $0.1$ & $0.1$ & $6.1$ & $5.8$ & $4.7$ & $0.1$ & $0.1$\\
\clasp & $8.1$ & $9.4$ & $7.0$ & -- & -- & $7.9$ & $8.8$ & $6.5$ & -- & --\\
\sparrow & $0.7$ & $0.7$ & $1.0$ & -- & -- & $2.7$ & $0.3$ & $0.9$ & -- & --\\
\midrule
 \multicolumn{11}{c}{CSSC-unsat-unif-k5-300s-2day}\\
\midrule
\clasp & $2.3$ & $2.4$ & $2.5$ & -- & -- & $2.3$ & $2.4$ & $2.5$ & -- & --\\
\sparrow & $96.2$ & $96.6$ & $105.6$ & -- & -- & $94.1$ & $95.8$ & $103.3$ & -- & --\\
\riss & $1.9$ & $1.9$ & $1.9$ & $1.3$ & $1.5$ & $10.6$ & $10.9$ & $11.1$ & $7.4$ & $8.6$\\
\minisathack & $2.2$ & $2.2$ & $2.2$ & $2.2$ & $2.2$ & $2.2$ & $2.2$ & $2.2$ & $2.1$ & $2.2$\\
\dccsat & $5.0$ & $5.0$ & $5.0$ & $5.0$ & $5.0$ & $5.4$ & $5.4$ & $5.4$ & $5.4$ & $5.4$\\
\bottomrule[1pt]
\end{tabular}
\caption{CSSC'14: \random}
\end{table}
\begin{table}[th]
\sffamily\small\centering
\setlength\tabcolsep{0.3em}
\begin{tabular}{l | ccccc | ccccc}
\toprule[1pt]
 & \multicolumn{5}{c|}{Training} & \multicolumn{5}{c}{Test}\\
 & \smac{}-d & \smac{}-c & \pils{} & \gga{}-d & \gga{}-c & \smac{}-d & \smac{}-c & \pils{} & \gga{}-d & \gga{}-c  \\
\midrule
 \multicolumn{11}{c}{CSSC-3SAT1k-sat-300s-2day}\\
\midrule
\minisathack & $1.0$ & $1.0$ & $1.0$ & $1.0$ & $1.0$ & $1.0$ & $1.0$ & $1.0$ & $1.0$ & $1.0$\\
\probsat & $32.3$ & $24.5$ & $32.2$ & -- & -- & $18.6$ & $5.7$ & $18.6$ & -- & --\\
\clasp & $1.0$ & $1.0$ & $1.0$ & -- & -- & $1.0$ & $1.0$ & $1.0$ & -- & --\\
\csccsat & $3.5$ & $3.5$ & $3.5$ & $1.0$ & $1.0$ & $0.9$ & $0.9$ & $0.9$ & $1.0$ & $1.0$\\
\yalsat & $6.5$ & $1.7$ & $8.6$ & $0.0$ & $0.7$ & $1.0$ & $0.6$ & $0.3$ & $0.0$ & $0.3$\\
\sparrow & $5.6$ & $26.8$ & $14.2$ & -- & -- & $1.8$ & $4.3$ & $1.2$ & -- & --\\
\midrule
 \multicolumn{11}{c}{CSSC-7SAT90-sat-300s-2day}\\
\midrule
\minisathack & $1.0$ & $1.0$ & $1.0$ & $1.0$ & $1.0$ & $1.0$ & $1.0$ & $1.0$ & $1.0$ & $1.0$\\
\probsat & $18.1$ & $13.3$ & $13.6$ & -- & -- & $22.9$ & $20.2$ & $21.0$ & -- & --\\
\clasp & $36.7$ & $1.0$ & $1.0$ & -- & -- & $1.0$ & $1.0$ & $1.0$ & -- & --\\
\csccsat & $1.6$ & $1.6$ & $1.6$ & $1.6$ & $1.6$ & $0.3$ & $0.3$ & $0.3$ & $0.3$ & $0.3$\\
\yalsat & $1.0$ & $1.3$ & $1.9$ & $1.0$ & $0.6$ & $1.6$ & $4.3$ & $1.1$ & $1.0$ & $1.8$\\
\sparrow & $15.9$ & $7.3$ & $2.5$ & -- & -- & $1.3$ & $5.5$ & $0.9$ & -- & --\\
\midrule
 \multicolumn{11}{c}{CSSC-5SAT500-sat-300s-2day}\\
\midrule
\minisathack & $1.0$ & $1.0$ & $1.0$ & $1.0$ & $1.0$ & $1.0$ & $1.0$ & $1.0$ & $1.0$ & $1.0$\\
\probsat & $1506.8$ & $1597.3$ & $1499.7$ & -- & -- & $1380.8$ & $1526.2$ & $1374.8$ & -- & --\\
\clasp & $1.0$ & $1.0$ & $1.0$ & -- & -- & $1.0$ & $1.0$ & $1.0$ & -- & --\\
\csccsat & $1.0$ & $1.0$ & $1.0$ & $0.1$ & $1.0$ & $1.0$ & $1.0$ & $1.0$ & $0.2$ & $1.0$\\
\yalsat & $1.5$ & $1.5$ & $1.2$ & $1.3$ & $1.1$ & $1.1$ & $1.1$ & $1.0$ & $1.0$ & $0.7$\\
\sparrow & $456.6$ & $358.2$ & $104.1$ & -- & -- & $481.3$ & $323.9$ & $100.3$ & -- & --\\
\bottomrule[1pt]
\end{tabular}
\caption{CSSC'14: \randomsat}
\end{table}
\begin{table}[th]
\sffamily\small\centering
\setlength\tabcolsep{0.3em}
\begin{tabular}{l | ccccc | ccccc}
\toprule[1pt]
 & \multicolumn{5}{c|}{Training} & \multicolumn{5}{c}{Test}\\
 & \smac{}-d & \smac{}-c & \pils{} & \gga{}-d & \gga{}-c & \smac{}-d & \smac{}-c & \pils{} & \gga{}-d & \gga{}-c  \\
\midrule
 \multicolumn{11}{c}{CSSC-CircuitFuzz-300s-2day}\\
\midrule
\minisathack & $2.9$ & $3.1$ & $1.9$ & $0.8$ & -- & $2.3$ & $1.6$ & $4.1$ & $4.3$ & --\\
\riss & $3.4$ & $2.1$ & $2.9$ & $0.6$ & $0.5$ & $0.7$ & $1.1$ & $1.5$ & $0.6$ & $0.4$\\
\clasp & $3.8$ & $3.1$ & $2.2$ & -- & -- & $4.7$ & $1.8$ & $1.3$ & -- & --\\
\cryptominisat & $7.3$ & $7.7$ & $4.2$ & $3.1$ & $7.0$ & $7.2$ & $8.0$ & $4.2$ & $2.7$ & $4.0$\\
\lingeling & $6.0$ & $2.7$ & $9.0$ & -- & $0.0$ & $5.0$ & $2.0$ & $4.6$ & -- & $0.0$\\
\sparrow & $9.6$ & $14.9$ & $9.8$ & -- & -- & $8.2$ & $6.8$ & $6.6$ & -- & --\\
\midrule
 \multicolumn{11}{c}{CSSC-IBM-300s-2day}\\
\midrule
\minisathack & $1.1$ & $2.8$ & $1.1$ & $0.9$ & $2.7$ & $3.0$ & $1.3$ & $1.1$ & $0.9$ & $0.1$\\
\riss & $1.0$ & $1.0$ & $0.5$ & $0.5$ & $0.1$ & $1.1$ & $2.6$ & $1.1$ & $2.3$ & $2.5$\\
\clasp & $2.5$ & $3.0$ & $2.7$ & -- & -- & $0.4$ & $1.1$ & $1.3$ & -- & --\\
\cryptominisat & $1.0$ & $1.5$ & $1.1$ & $0.2$ & $0.6$ & $1.1$ & $1.8$ & $1.7$ & $0.4$ & $1.0$\\
\lingeling & $1.0$ & $0.9$ & $1.0$ & -- & $0.0$ & $1.1$ & $1.0$ & $1.4$ & -- & $0.0$\\
\sparrow & $4.1$ & $8.2$ & $1.0$ & -- & -- & $8.8$ & $9.7$ & $0.9$ & -- & --\\
\midrule
 \multicolumn{11}{c}{CSSC-BMC08-300s-2day}\\
\midrule
\minisathack & $2.0$ & $2.1$ & $2.0$ & $3.0$ & $0.5$ & $0.6$ & $1.8$ & $0.7$ & $1.1$ & $1.8$\\
\riss & $2.3$ & $2.5$ & $1.3$ & $0.6$ & -- & $1.6$ & $1.3$ & $1.0$ & $0.5$ & --\\
\clasp & $4.2$ & $5.4$ & $1.2$ & -- & -- & $4.8$ & $5.9$ & $1.5$ & -- & --\\
\cryptominisat & $1.0$ & $1.1$ & $0.6$ & $0.3$ & $0.7$ & $1.9$ & $1.3$ & $1.9$ & $0.4$ & $0.0$\\
\lingeling & $1.7$ & $1.7$ & $2.0$ & -- & $0.1$ & $1.1$ & $1.0$ & $1.0$ & -- & $0.1$\\
\sparrow & $8.9$ & $8.3$ & $4.9$ & -- & -- & $8.0$ & $5.3$ & $4.0$ & -- & --\\
\bottomrule[1pt]
\end{tabular}
\caption{CSSC'14: \indu}
\end{table}
\begin{table}[th]
\sffamily\small\centering
\setlength\tabcolsep{0.3em}
\begin{tabular}{l | ccccc | ccccc}
\toprule[1pt]
 & \multicolumn{5}{c|}{Training} & \multicolumn{5}{c}{Test}\\
 & \smac{}-d & \smac{}-c & \pils{} & \gga{}-d & \gga{}-c & \smac{}-d & \smac{}-c & \pils{} & \gga{}-d & \gga{}-c  \\
\midrule
 \multicolumn{11}{c}{CSSC-LABS-300s-2day}\\
\midrule
\minisathack & $1.2$ & $1.6$ & $2.4$ & $1.2$ & -- & $1.1$ & $1.3$ & $1.0$ & $0.8$ & --\\
\riss & $1.1$ & $1.9$ & $2.5$ & $0.0$ & $0.5$ & $0.4$ & $1.1$ & $2.0$ & $0.1$ & $0.3$\\
\yalsat & $2.4$ & $3.6$ & $1.0$ & -- & $0.0$ & $1.8$ & $14.5$ & $1.0$ & -- & $0.0$\\
\clasp & $0.3$ & $0.2$ & $0.8$ & -- & -- & $0.3$ & $2.6$ & $0.3$ & -- & --\\
\cryptominisat & $2.1$ & $0.9$ & $1.3$ & $0.5$ & $0.6$ & $2.5$ & $1.3$ & $0.6$ & $0.2$ & $0.7$\\
\lingeling & $0.8$ & $0.6$ & $0.5$ & -- & $0.0$ & $0.5$ & $1.9$ & $0.4$ & -- & $0.6$\\
\sparrow & $3.2$ & $4.4$ & $3.1$ & -- & -- & $1.9$ & $4.8$ & $4.7$ & -- & --\\
\midrule
 \multicolumn{11}{c}{CSSC-GI-300s-2day}\\
\midrule
\minisathack & $2.5$ & $2.4$ & $2.4$ & -- & $1.3$ & $1.3$ & $1.4$ & $1.4$ & -- & $1.3$\\
\riss & $9.1$ & $7.4$ & $2.9$ & $0.2$ & $0.5$ & $9.0$ & $10.6$ & $3.2$ & $0.3$ & $0.0$\\
\lingeling & $0.9$ & $4.1$ & $1.0$ & -- & $0.0$ & $0.8$ & $4.5$ & $1.0$ & -- & $0.0$\\
\clasp & $18.5$ & $18.1$ & $7.5$ & -- & -- & $20.5$ & $23.3$ & $12.0$ & -- & --\\
\cryptominisat & $5.5$ & $4.8$ & $5.8$ & $2.1$ & $0.0$ & $11.5$ & $11.3$ & $11.1$ & $8.5$ & $1.6$\\
\yalsat & $3.1$ & $0.2$ & $0.2$ & $0.1$ & $0.0$ & $2.1$ & $6.2$ & $0.8$ & $0.1$ & $0.0$\\
\sparrow & $11.8$ & $11.7$ & $11.4$ & -- & -- & $14.8$ & $15.4$ & $15.4$ & -- & --\\
\midrule
 \multicolumn{11}{c}{CSSC-Queens-300s-2day}\\
\midrule
\minisathack & $1.2$ & $1.2$ & $1.3$ & $1.3$ & $1.1$ & $1.4$ & $1.3$ & $1.4$ & $1.4$ & $1.1$\\
\riss & $4.9$ & $4.0$ & $2.4$ & $0.4$ & $0.2$ & $4.0$ & $3.4$ & $2.1$ & $0.4$ & $0.2$\\
\lingeling & $1.9$ & $1.1$ & $2.4$ & -- & $0.0$ & $2.8$ & $2.4$ & $2.9$ & -- & $0.0$\\
\clasp & $100.7$ & $110.4$ & $48.0$ & -- & -- & $144.3$ & $150.5$ & $61.4$ & -- & --\\
\cryptominisat & $4.7$ & $4.3$ & $3.5$ & $2.0$ & $2.9$ & $3.4$ & $1.6$ & $2.3$ & $1.3$ & $1.8$\\
\yalsat & $1.0$ & $1.0$ & $1.0$ & -- & -- & $1.0$ & $1.0$ & $1.0$ & -- & --\\
\sparrow & $20.5$ & $19.6$ & $5.7$ & -- & -- & $13.5$ & $11.9$ & $5.2$ & -- & --\\
\bottomrule[1pt]
\end{tabular}
\caption{CSSC'14: \crafted}
\end{table}

%%%%%%%%%%%%%%%%%%%%%%%%%%%%%%%%%%%%%%%%%%%%%%%%%%%%%%%%%%%%%%%%
%%% CSSC13
%%%%%%%%%%%%%%%%%%%%%%%%%%%%%%%%%%%%%%%%%%%%%%%%%%%%%%%%%%%%%%%%

%INDUSTRIAL

\begin{table}[h]
\footnotesize
\begin{tabular}{l | cccc | cccc | l}
\hline\hline
 & \multicolumn{4}{c|}{Training performance} & \multicolumn{4}{c|}{Test performance} & \\
Solver & \multicolumn{2}{c}{$\#$Timeouts}  & \multicolumn{2}{c|}{PAR1} & \multicolumn{2}{c}{$\#$Timeouts}  & \multicolumn{2}{c|}{PAR1} & Configurator\\
 & default & config. & default & config. & default & config. & default & config. & \\ 
\hline
\rissgExt & $82$ & $67$ & $71.54$ & $65.65$ & $70$ & $\mathbf{46}$ & $74.43$ & $\mathbf{58.39}$ & smac-2\\
\lingeling & $81$ & $\mathbf{80}$ & $73.87$ & $73.31$ & $69$ & $69$ & $77.22$ & $\mathbf{75.30}$ & paramils-1\\
\rissg & $82$ & $82$ & $71.42$ & $\mathbf{70.10}$ & $70$ & $\mathbf{69}$ & $74.63$ & $\mathbf{72.99}$ & paramils-4\\
\SolverFourtyThree & $91$ & $\mathbf{90}$ & $77.28$ & $77.14$ & $77$ & $77$ & $82.55$ & $\mathbf{80.32}$ & paramils-1-\\
\forlnodrup & $83$ & $\mathbf{82}$ & $79.42$ & $\mathbf{74.83}$ & $69$ & $69$ & $80.81$ & $\mathbf{75.61}$ & smac-3\\
\simpsat & $84$ & $\mathbf{82}$ & $77.14$ & $77.38$ & $70$ & $\mathbf{69}$ & $79.41$ & $78.99$ & paramils-2\\
\clasp-cssc & $86$ & $\mathbf{84}$ & $75.36$ & $\mathbf{71.85}$ & $71$ & $71$ & $77.71$ & $\mathbf{75.32}$ & smac-2\\
\satj & $98$ & $98$ & $92.48$ & $92.05$ & $77$ & $\mathbf{76}$ & $89.81$ & $\mathbf{87.18}$ & smac-4\\
\gnoveltyGCwa & $371$ & $371$ & $291.39$ & $291.39$ & $295$ & $295$ & $293.08$ & $293.07$ & smac-2\\
\gnoveltyPCL & $373$ & $\mathbf{371}$ & $293.17$ & $\mathbf{291.43}$ & $295$ & $\mathbf{294}$ & $293.74$ & $292.96$ & smac-2\\
\gnoveltyGCa & $371$ & $371$ & $291.39$ & $291.39$ & $295$ & $295$ & $293.07$ & $293.07$ & smac-0\\
\hline\hline
\end{tabular}
\caption{CSSC13: Track: \indu; Benchmarks: \hw}
\end{table}

\begin{table}[h]
\footnotesize
\begin{tabular}{l | cccc | cccc | l}
\hline\hline
 & \multicolumn{4}{c|}{Training performance} & \multicolumn{4}{c|}{Test performance} & \\
Solver & \multicolumn{2}{c}{$\#$Timeouts}  & \multicolumn{2}{c|}{PAR1} & \multicolumn{2}{c}{$\#$Timeouts}  & \multicolumn{2}{c|}{PAR1} & Configurator\\
 & default & config. & default & config. & default & config. & default & config. & \\ 
\hline
\rissgExt & $19$ & $\mathbf{11}$ & $33.49$ & $\mathbf{25.62}$ & $21$ & $\mathbf{16}$ & $38.86$ & $\mathbf{31.35}$ & paramils-1\\
\lingeling & $36$ & $\mathbf{12}$ & $54.07$ & $\mathbf{29.13}$ & $39$ & $\mathbf{20}$ & $60.62$ & $\mathbf{35.31}$ & smac-4\\
\rissg & $19$ & $\mathbf{11}$ & $33.17$ & $\mathbf{26.90}$ & $20$ & $18$ & $38.38$ & $\mathbf{33.12}$ & smac-4\\
\SolverFourtyThree & $19$ & $\mathbf{11}$ & $32.32$ & $\mathbf{27.45}$ & $20$ & $20$ & $36.85$ & $38.06$ & paramils-1\\
\forlnodrup & $29$ & $\mathbf{15}$ & $45.07$ & $\mathbf{33.91}$ & $33$ & $\mathbf{23}$ & $51.04$ & $\mathbf{41.74}$ & paramils-4\\
\simpsat & $25$ & $\mathbf{21}$ & $40.23$ & $39.22$ & $26$ & $\mathbf{24}$ & $47.16$ & $45.28$ & smac-2\\
\clasp-cssc & $23$ & $\mathbf{7}$ & $37.04$ & $\mathbf{20.97}$ & $26$ & $\mathbf{17}$ & $45.36$ & $\mathbf{28.62}$ & paramils-3\\
\satj & $29$ & $\mathbf{24}$ & $47.24$ & $46.56$ & $36$ & $\mathbf{30}$ & $58.98$ & $\mathbf{51.31}$ & paramils-1\\
\gnoveltyGCwa & $296$ & $\mathbf{292}$ & $299.52$ & $\mathbf{295.55}$ & $301$ & $\mathbf{295}$ & $299.60$ & $\mathbf{296.00}$ & smac-1\\
\gnoveltyPCL & $299$ & $299$ & $300.00$ & $300.00$ & $302$ & $302$ & $300.00$ & $300.00$ & smac-4\\
\gnoveltyGCa & $297$ & $295$ & $298.41$ & $297.98$ & $\mathbf{300}$ & $302$ & $\mathbf{298.97}$ & $300.00$ & paramils-2\\
\hline\hline
\end{tabular}
\caption{CSSC13: Track: \indu; Benchmarks: \circuit}
\end{table}

\begin{table}[h]
\footnotesize
\begin{tabular}{l | cccc | cccc | l}
\hline\hline
 & \multicolumn{4}{c|}{Training performance} & \multicolumn{4}{c|}{Test performance} & \\
Solver & \multicolumn{2}{c}{$\#$Timeouts}  & \multicolumn{2}{c|}{PAR1} & \multicolumn{2}{c}{$\#$Timeouts}  & \multicolumn{2}{c|}{PAR1} & Configurator\\
 & default & config. & default & config. & default & config. & default & config. & \\ 
\hline
\rissgExt & $157$ & $\mathbf{51}$ & $74.73$ & $\mathbf{24.34}$ & $32$ & $\mathbf{20}$ & $46.15$ & $\mathbf{22.36}$ & smac-0\\
\lingeling & $139$ & $137$ & $76.43$ & $76.87$ & $28$ & $\mathbf{26}$ & $51.96$ & $\mathbf{49.71}$ & paramils-1\\
\rissg & $156$ & $\mathbf{144}$ & $75.19$ & $75.62$ & $32$ & $30$ & $46.39$ & $46.47$ & smac-1\\
\SolverFourtyThree & $142$ & $142$ & $77.70$ & $77.70$ & $30$ & $30$ & $52.51$ & $52.51$ & smac-1\\
\forlnodrup & $187$ & $\mathbf{173}$ & $104.62$ & $\mathbf{92.38}$ & $50$ & $\mathbf{36}$ & $81.92$ & $\mathbf{63.10}$ & smac-2\\
\simpsat & $175$ & $173$ & $\mathbf{96.62}$ & $98.03$ & $38$ & $35$ & $71.58$ & $70.42$ & paramils-4\\
\clasp-cssc & $213$ & $\mathbf{191}$ & $92.58$ & $\mathbf{86.49}$ & $66$ & $\mathbf{42}$ & $77.21$ & $\mathbf{60.67}$ & smac-3\\
\satj & $257$ & $256$ & $123.72$ & $125.42$ & $70$ & $70$ & $99.14$ & $99.87$ & smac-3\\
\gnoveltyGCwa & $768$ & $\mathbf{753}$ & $286.13$ & $\mathbf{282.89}$ & $291$ & $\mathbf{285}$ & $289.64$ & $\mathbf{286.42}$ & smac-1\\
\gnoveltyPCL & $770$ & $\mathbf{755}$ & $286.61$ & $\mathbf{282.71}$ & $289$ & $\mathbf{288}$ & $288.37$ & $287.80$ & paramils-3\\
\gnoveltyGCa & $774$ & $\mathbf{763}$ & $288.01$ & $\mathbf{284.62}$ & $291$ & $290$ & $289.67$ & $288.30$ & smac-0\\
\hline\hline
\end{tabular}
\caption{CSSC13: Track: \indu; Benchmarks: \bmc}
\end{table}

\begin{table}[h]
\footnotesize
\begin{tabular}{l | cccc | cccc | l}
\hline\hline
 & \multicolumn{4}{c|}{Training performance} & \multicolumn{4}{c|}{Test performance} & \\
Solver & \multicolumn{2}{c}{$\#$Timeouts}  & \multicolumn{2}{c|}{PAR1} & \multicolumn{2}{c}{$\#$Timeouts}  & \multicolumn{2}{c|}{PAR1} & Configurator\\
 & default & config. & default & config. & default & config. & default & config. & \\ 
\hline
\rissgExt & $0$ & $0$ & $0.65$ & $\mathbf{0.12}$ & $0$ & $0$ & $0.57$ & $\mathbf{0.11}$ & smac-3\\
\lingeling & $1$ & $\mathbf{0}$ & $6.13$ & $\mathbf{0.16}$ & $0$ & $0$ & $3.32$ & $\mathbf{0.16}$ & smac-3\\
\rissg & $0$ & $0$ & $0.71$ & $\mathbf{0.42}$ & $0$ & $0$ & $0.61$ & $\mathbf{0.40}$ & smac-3\\
\SolverFourtyThree & $0$ & $0$ & $6.27$ & $\mathbf{2.60}$ & $0$ & $0$ & $6.00$ & $\mathbf{2.39}$ & smac-0\\
\forlnodrup & $0$ & $0$ & $4.56$ & $\mathbf{0.66}$ & $0$ & $0$ & $3.71$ & $\mathbf{0.59}$ & smac-1\\
\simpsat & $0$ & $0$ & $6.32$ & $\mathbf{5.27}$ & $0$ & $0$ & $4.64$ & $4.97$ & smac-0\\
\clasp-cssc & $0$ & $0$ & $0.52$ & $\mathbf{0.12}$ & $0$ & $0$ & $0.44$ & $\mathbf{0.11}$ & smac-0\\
\satj & $1$ & $\mathbf{0}$ & $6.28$ & $\mathbf{3.11}$ & $1$ & $\mathbf{0}$ & $7.32$ & $\mathbf{2.99}$ & smac-0\\
\gnoveltyGCwa & $250$ & $\mathbf{235}$ & $248.96$ & $\mathbf{234.72}$ & $244$ & $\mathbf{215}$ & $243.06$ & $\mathbf{216.63}$ & smac-4\\
\gnoveltyPCL & $235$ & $\mathbf{234}$ & $234.40$ & $233.61$ & $215$ & $215$ & $216.58$ & $\mathbf{214.43}$ & smac-2\\
\gnoveltyGCa & $251$ & $\mathbf{235}$ & $250.68$ & $\mathbf{237.95}$ & $243$ & $\mathbf{217}$ & $243.69$ & $\mathbf{219.09}$ & smac-2\\
\hline\hline
\end{tabular}
\caption{CSSC13: Track: \indu; Benchmarks: \swv}
\end{table}

% CRAFTED
\clearpage

\begin{table}[h]
\footnotesize
\begin{tabular}{l | cccc | cccc | l}
\hline\hline
 & \multicolumn{4}{c|}{Training performance} & \multicolumn{4}{c|}{Test performance} & \\
Solver & \multicolumn{2}{c}{$\#$Timeouts}  & \multicolumn{2}{c|}{PAR1} & \multicolumn{2}{c}{$\#$Timeouts}  & \multicolumn{2}{c|}{PAR1} & Configurator\\
 & default & config. & default & config. & default & config. & default & config. & \\ 
\hline
\rissgExt & $89$ & $\mathbf{42}$ & $84.32$ & $\mathbf{49.21}$ & $98$ & $\mathbf{42}$ & $90.94$ & $\mathbf{44.14}$ & smac-1\\
\clasp-cssc & $90$ & $88$ & $84.97$ & $83.53$ & $97$ & $\mathbf{90}$ & $91.25$ & $\mathbf{86.96}$ & smac-2\\
\forlnodrup & $92$ & $\mathbf{88}$ & $87.92$ & $\mathbf{84.50}$ & $95$ & $91$ & $91.19$ & $\mathbf{87.25}$ & paramils-0\\
\lingeling & $95$ & $92$ & $91.84$ & $\mathbf{87.62}$ & $105$ & $\mathbf{97}$ & $99.20$ & $\mathbf{92.07}$ & smac-4\\
\rissg & $91$ & $87$ & $84.54$ & $84.56$ & $97$ & $\mathbf{89}$ & $91.57$ & $\mathbf{85.09}$ & smac-1\\
\simpsat & $101$ & $101$ & $\mathbf{93.44}$ & $93.77$ & $107$ & $107$ & $100.35$ & $100.35$ & paramils-1\\
\SolverFourtyThree & $85$ & $84$ & $82.56$ & $83.85$ & $90$ & $87$ & $88.19$ & $85.55$ & smac-4\\
\satj & $103$ & $\mathbf{95}$ & $101.86$ & $\mathbf{92.14}$ & $110$ & $\mathbf{104}$ & $104.55$ & $\mathbf{96.62}$ & smac-4\\
\gnoveltyGCwa & $190$ & $\mathbf{149}$ & $168.46$ & $\mathbf{144.75}$ & $195$ & $\mathbf{154}$ & $168.56$ & $\mathbf{144.51}$ & paramils-4\\
\gnoveltyGCa & $242$ & $\mathbf{178}$ & $214.66$ & $\mathbf{158.37}$ & $240$ & $\mathbf{173}$ & $207.66$ & $\mathbf{153.91}$ & paramils-4\\
\gnoveltyPCL & $197$ & $\mathbf{188}$ & $175.15$ & $\mathbf{166.51}$ & $199$ & $\mathbf{183}$ & $175.98$ & $\mathbf{163.43}$ & paramils-0\\
\hline\hline
\end{tabular}
\caption{CSSC13: Track: \crafted; Benchmarks: \labs}
\end{table}

\begin{table}[h]
\footnotesize
\begin{tabular}{l | cccc | cccc | l}
\hline\hline
 & \multicolumn{4}{c|}{Training performance} & \multicolumn{4}{c|}{Test performance} & \\
Solver & \multicolumn{2}{c}{$\#$Timeouts}  & \multicolumn{2}{c|}{PAR1} & \multicolumn{2}{c}{$\#$Timeouts}  & \multicolumn{2}{c|}{PAR1} & Configurator\\
 & default & config. & default & config. & default & config. & default & config. & \\ 
\hline
\rissgExt & $143$ & $\mathbf{2}$ & $46.48$ & $\mathbf{1.15}$ & $50$ & $\mathbf{2}$ & $46.74$ & $\mathbf{2.29}$ & smac-0\\
\clasp-cssc & $131$ & $\mathbf{33}$ & $41.81$ & $\mathbf{22.42}$ & $42$ & $\mathbf{6}$ & $38.94$ & $\mathbf{19.04}$ & smac-2\\
\forlnodrup & $115$ & $\mathbf{36}$ & $41.74$ & $\mathbf{26.23}$ & $40$ & $\mathbf{7}$ & $40.36$ & $\mathbf{22.79}$ & smac-0\\
\lingeling & $131$ & $\mathbf{32}$ & $40.77$ & $\mathbf{19.84}$ & $43$ & $\mathbf{10}$ & $39.15$ & $\mathbf{17.61}$ & smac-4\\
\rissg & $143$ & $\mathbf{128}$ & $46.57$ & $\mathbf{42.33}$ & $51$ & $\mathbf{42}$ & $46.80$ & $\mathbf{39.11}$ & smac-0\\
\simpsat & $124$ & $124$ & $42.15$ & $42.15$ & $42$ & $42$ & $42.54$ & $42.54$ & paramils-3\\
\SolverFourtyThree & $202$ & $\mathbf{194}$ & $66.51$ & $\mathbf{60.35}$ & $66$ & $\mathbf{65}$ & $61.86$ & $\mathbf{58.13}$ & smac-2\\
\satj & $182$ & $\mathbf{159}$ & $58.48$ & $\mathbf{52.31}$ & $62$ & $\mathbf{57}$ & $56.68$ & $\mathbf{52.46}$ & paramils-3\\
\gnoveltyGCwa & $578$ & $578$ & $169.94$ & $\mathbf{169.25}$ & $180$ & $180$ & $155.99$ & $\mathbf{154.94}$ & smac-4\\
\gnoveltyGCa & $592$ & $\mathbf{578}$ & $173.28$ & $\mathbf{169.21}$ & $183$ & $\mathbf{180}$ & $157.64$ & $\mathbf{154.89}$ & paramils-2\\
\gnoveltyPCL & $599$ & $\mathbf{582}$ & $176.70$ & $\mathbf{173.52}$ & $179$ & $178$ & $158.20$ & $156.79$ & smac-4\\
\hline\hline
\end{tabular}
\caption{CSSC13: Track: \crafted; Benchmarks: \gi}
\end{table}

% RANDOM
\clearpage

\begin{table}[h]
\footnotesize
\begin{tabular}{l | cccc | cccc | l}
\hline\hline
 & \multicolumn{4}{c|}{Training performance} & \multicolumn{4}{c|}{Test performance} & \\
Solver & \multicolumn{2}{c}{$\#$Timeouts}  & \multicolumn{2}{c|}{PAR1} & \multicolumn{2}{c}{$\#$Timeouts}  & \multicolumn{2}{c|}{PAR1} & Configurator\\
 & default & config. & default & config. & default & config. & default & config. & \\ 
\hline
\clasp-cssc & $250$ & $250$ & $300.00$ & $300.00$ & $250$ & $250$ & $300.00$ & $300.00$ & paramils-4\\
\lingeling & $250$ & $250$ & $300.00$ & $300.00$ & $250$ & $250$ & $300.00$ & $300.00$ & paramils-4\\
\rissgExt & $250$ & $250$ & $300.00$ & $300.00$ & $250$ & $250$ & $300.00$ & $300.00$ & smac-3\\
\rissg & $250$ & $250$ & $300.00$ & $300.00$ & $250$ & $250$ & $300.00$ & $300.00$ & smac-0\\
\SolverFourtyThree & $250$ & $250$ & $300.00$ & $300.00$ & $250$ & $250$ & $300.00$ & $300.00$ & paramils-0\\
\simpsat & $250$ & $250$ & $300.00$ & $300.00$ & $250$ & $250$ & $300.00$ & $300.00$ & smac-4\\
\satj & $250$ & $250$ & $300.00$ & $300.00$ & $250$ & $250$ & $300.00$ & $300.00$ & paramils-1\\
\forlnodrup & $250$ & $250$ & $300.00$ & $300.00$ & $250$ & $250$ & $300.00$ & $300.00$ & paramils-4\\
\gnoveltyGCwa & $10$ & $\mathbf{0}$ & $43.31$ & $\mathbf{22.35}$ & $8$ & $\mathbf{1}$ & $42.91$ & $\mathbf{21.28}$ & paramils-3\\
\gnoveltyGCa & $158$ & $\mathbf{6}$ & $236.96$ & $\mathbf{38.48}$ & $163$ & $\mathbf{4}$ & $236.57$ & $\mathbf{33.91}$ & paramils-4\\
\gnoveltyPCL & $250$ & $\mathbf{10}$ & $300.00$ & $\mathbf{81.18}$ & $250$ & $\mathbf{11}$ & $300.00$ & $\mathbf{78.03}$ & smac-0\\
\hline\hline
\end{tabular}
\caption{CSSC13: Track: \random; Benchmarks: \fivesatfiveh}
\end{table}

\begin{table}[h]
\footnotesize
\begin{tabular}{l | cccc | cccc | l}
\hline\hline
 & \multicolumn{4}{c|}{Training performance} & \multicolumn{4}{c|}{Test performance} & \\
Solver & \multicolumn{2}{c}{$\#$Timeouts}  & \multicolumn{2}{c|}{PAR1} & \multicolumn{2}{c}{$\#$Timeouts}  & \multicolumn{2}{c|}{PAR1} & Configurator\\
 & default & config. & default & config. & default & config. & default & config. & \\ 
\hline
\clasp-cssc & $0$ & $0$ & $1.45$ & $\mathbf{0.37}$ & $0$ & $0$ & $1.44$ & $\mathbf{0.37}$ & paramils-3\\
\lingeling & $0$ & $0$ & $1.60$ & $\mathbf{0.54}$ & $0$ & $0$ & $1.61$ & $\mathbf{0.54}$ & smac-0\\
\rissgExt & $0$ & $0$ & $0.96$ & $\mathbf{0.53}$ & $0$ & $0$ & $0.95$ & $\mathbf{0.53}$ & paramils-0\\
\rissg & $0$ & $0$ & $0.95$ & $\mathbf{0.60}$ & $0$ & $0$ & $0.94$ & $\mathbf{0.60}$ & paramils-4\\
\SolverFourtyThree & $0$ & $0$ & $0.84$ & $\mathbf{0.73}$ & $0$ & $0$ & $0.82$ & $\mathbf{0.72}$ & smac-3\\
\simpsat & $0$ & $0$ & $2.62$ & $2.61$ & $0$ & $0$ & $2.59$ & $\mathbf{2.59}$ & smac-4\\
\satj & $0$ & $0$ & $4.87$ & $\mathbf{4.31}$ & $0$ & $0$ & $4.80$ & $\mathbf{4.40}$ & paramils-3\\
\forlnodrup & $0$ & $0$ & $4.32$ & $\mathbf{1.25}$ & $0$ & $0$ & $4.24$ & $\mathbf{1.24}$ & smac-1\\
\gnoveltyGCwa & $300$ & $300$ & $300.00$ & $300.00$ & $250$ & $250$ & $300.00$ & $300.00$ & paramils-1\\
\gnoveltyGCa & $300$ & $300$ & $300.00$ & $300.00$ & $250$ & $250$ & $300.00$ & $300.00$ & paramils-2\\
\gnoveltyPCL & $300$ & $300$ & $300.00$ & $300.00$ & $250$ & $250$ & $300.00$ & $300.00$ & smac-4\\
\hline\hline
\end{tabular}
\caption{CSSC13: Track: \random; Benchmarks: \unif}
\end{table}

\begin{table}[h]
\footnotesize
\begin{tabular}{l | cccc | cccc | l}
\hline\hline
 & \multicolumn{4}{c|}{Training performance} & \multicolumn{4}{c|}{Test performance} & \\
Solver & \multicolumn{2}{c}{$\#$Timeouts}  & \multicolumn{2}{c|}{PAR1} & \multicolumn{2}{c}{$\#$Timeouts}  & \multicolumn{2}{c|}{PAR1} & Configurator\\
 & default & config. & default & config. & default & config. & default & config. & \\ 
\hline
\clasp-cssc & $25$ & $\mathbf{0}$ & $53.74$ & $\mathbf{4.23}$ & $11$ & $\mathbf{0}$ & $39.33$ & $\mathbf{2.79}$ & smac-0\\
\lingeling & $20$ & $\mathbf{0}$ & $46.42$ & $\mathbf{9.51}$ & $8$ & $\mathbf{0}$ & $34.05$ & $\mathbf{7.86}$ & smac-2\\
\rissgExt & $15$ & $\mathbf{0}$ & $40.97$ & $\mathbf{19.74}$ & $11$ & $\mathbf{0}$ & $33.77$ & $\mathbf{13.86}$ & smac-1\\
\rissg & $15$ & $\mathbf{0}$ & $40.31$ & $\mathbf{17.65}$ & $10$ & $\mathbf{0}$ & $33.61$ & $\mathbf{14.76}$ & smac-4\\
\SolverFourtyThree & $15$ & $\mathbf{8}$ & $38.64$ & $37.02$ & $6$ & $\mathbf{3}$ & $28.78$ & $27.38$ & smac-3\\
\simpsat & $12$ & $\mathbf{10}$ & $39.54$ & $39.52$ & $4$ & $4$ & $29.88$ & $29.69$ & smac-3\\
\satj & $19$ & $\mathbf{11}$ & $50.34$ & $\mathbf{44.26}$ & $7$ & $5$ & $35.81$ & $\mathbf{31.21}$ & smac-4\\
\forlnodrup & $57$ & $\mathbf{15}$ & $83.13$ & $\mathbf{43.54}$ & $39$ & $\mathbf{8}$ & $69.75$ & $\mathbf{31.19}$ & smac-4\\
\gnoveltyGCwa & $162$ & $162$ & $162.02$ & $\mathbf{162.01}$ & $124$ & $124$ & $148.82$ & $148.82$ & smac-1\\
\gnoveltyGCa & $162$ & $162$ & $162.01$ & $162.01$ & $124$ & $124$ & $148.82$ & $148.82$ & paramils-2\\
\gnoveltyPCL & $162$ & $162$ & $162.04$ & $\mathbf{162.02}$ & $124$ & $124$ & $148.86$ & $148.88$ & paramils-4\\
\hline\hline
\end{tabular}
\caption{CSSC13: Track: \random; Benchmarks: \kthree}
\end{table}

%%%%%%%%%%%%%%%%%%%%%%%%%%%%%%%%%%%%%%%%%%%%%%%%%%%%%%%%%%%%%%%%
%%% CSSC14
%%%%%%%%%%%%%%%%%%%%%%%%%%%%%%%%%%%%%%%%%%%%%%%%%%%%%%%%%%%%%%%%

%INDUSTRIAL
\clearpage

\begin{table}[h]
\footnotesize
\begin{tabular}{l | cccc | cccc | l}
\hline\hline
 & \multicolumn{4}{c|}{Training performance} & \multicolumn{4}{c|}{Test performance} & \\
Solver & \multicolumn{2}{c}{$\#$Timeouts}  & \multicolumn{2}{c|}{PAR1} & \multicolumn{2}{c}{$\#$Timeouts}  & \multicolumn{2}{c|}{PAR1} & Configurator\\
 & default & config. & default & config. & default & config. & default & config. & \\ 
\hline
\lingeling & $81$ & $81$ & $76.85$ & $76.41$ & $69$ & $69$ & $80.41$ & $\mathbf{77.16}$ & paramils-1\\
\minisathack & $82$ & $\mathbf{81}$ & $68.87$ & $\mathbf{68.01}$ & $70$ & $70$ & $72.91$ & $\mathbf{72.16}$ & smac-3\\
\clasp & $85$ & $\mathbf{84}$ & $74.11$ & $\mathbf{71.11}$ & $71$ & $71$ & $75.59$ & $75.24$ & smac-0\\
\riss & $82$ & $82$ & $\mathbf{72.28}$ & $72.49$ & $72$ & $72$ & $77.32$ & $\mathbf{76.83}$ & smac-disc-0\\
\cryptominisat & $81$ & $\mathbf{80}$ & $74.55$ & $75.26$ & $70$ & $\mathbf{69}$ & $77.48$ & $78.58$ & smac-1\\
\sparrow & $83$ & $\mathbf{82}$ & $152.12$ & $\mathbf{75.93}$ & $72$ & $72$ & $154.35$ & $\mathbf{80.03}$ & smac-1\\
\hline\hline
\end{tabular}
\caption{CSSC14: Track: \indu; Benchmarks: \hw}
\end{table}

\begin{table}[h]
\footnotesize
\begin{tabular}{l | cccc | cccc | l}
\hline\hline
 & \multicolumn{4}{c|}{Training performance} & \multicolumn{4}{c|}{Test performance} & \\
Solver & \multicolumn{2}{c}{$\#$Timeouts}  & \multicolumn{2}{c|}{PAR1} & \multicolumn{2}{c}{$\#$Timeouts}  & \multicolumn{2}{c|}{PAR1} & Configurator\\
 & default & config. & default & config. & default & config. & default & config. & \\ 
\hline
\lingeling & $23$ & $\mathbf{11}$ & $40.43$ & $\mathbf{26.38}$ & $30$ & $\mathbf{18}$ & $47.79$ & $\mathbf{31.96}$ & paramils-1\\
\minisathack & $13$ & $\mathbf{10}$ & $29.01$ & $\mathbf{24.97}$ & $21$ & $19$ & $38.45$ & $\mathbf{34.29}$ & smac-2\\
\clasp & $11$ & $\mathbf{7}$ & $24.87$ & $\mathbf{21.32}$ & $18$ & $\mathbf{12}$ & $32.60$ & $\mathbf{27.63}$ & smac-disc-1\\
\riss & $16$ & $\mathbf{12}$ & $33.88$ & $\mathbf{29.16}$ & $20$ & $22$ & $39.31$ & $37.21$ & smac-disc-1\\
\cryptominisat & $25$ & $\mathbf{14}$ & $39.13$ & $\mathbf{30.18}$ & $31$ & $\mathbf{20}$ & $51.26$ & $\mathbf{36.09}$ & smac-1\\
\sparrow & $26$ & $\mathbf{13}$ & $167.24$ & $\mathbf{32.40}$ & $29$ & $\mathbf{21}$ & $173.79$ & $\mathbf{39.67}$ & smac-disc-2\\
\hline\hline
\end{tabular}
\caption{CSSC14: Track: \indu; Benchmarks: \circuit}
\end{table}

\begin{table}[h]
\footnotesize
\begin{tabular}{l | cccc | cccc | l}
\hline\hline
 & \multicolumn{4}{c|}{Training performance} & \multicolumn{4}{c|}{Test performance} & \\
Solver & \multicolumn{2}{c}{$\#$Timeouts}  & \multicolumn{2}{c|}{PAR1} & \multicolumn{2}{c}{$\#$Timeouts}  & \multicolumn{2}{c|}{PAR1} & Configurator\\
 & default & config. & default & config. & default & config. & default & config. & \\ 
\hline
\lingeling & $115$ & $\mathbf{109}$ & $75.40$ & $\mathbf{73.62}$ & $20$ & $20$ & $43.65$ & $\mathbf{42.56}$ & paramils-1\\
\minisathack & $108$ & $\mathbf{100}$ & $62.12$ & $\mathbf{60.73}$ & $22$ & $22$ & $36.47$ & $\mathbf{34.87}$ & gga-disc-1\\
\clasp & $151$ & $\mathbf{134}$ & $79.57$ & $\mathbf{75.16}$ & $44$ & $\mathbf{30}$ & $57.75$ & $\mathbf{47.29}$ & smac-3\\
\riss & $172$ & $\mathbf{91}$ & $107.65$ & $\mathbf{70.43}$ & $39$ & $\mathbf{26}$ & $72.79$ & $\mathbf{52.62}$ & smac-disc-2\\
\cryptominisat & $147$ & $143$ & $\mathbf{96.32}$ & $103.54$ & $40$ & $37$ & $70.88$ & $74.47$ & smac-1\\
\sparrow & $217$ & $\mathbf{145}$ & $204.66$ & $\mathbf{87.96}$ & $62$ & $\mathbf{36}$ & $190.12$ & $\mathbf{60.85}$ & smac-2\\
\hline\hline
\end{tabular}
\caption{CSSC14: Track: \indu; Benchmarks: \bmc}
\end{table}

%CRAFTED 
\clearpage

\begin{table}[h]
\footnotesize
\begin{tabular}{l | cccc | cccc | l}
\hline\hline
 & \multicolumn{4}{c|}{Training performance} & \multicolumn{4}{c|}{Test performance} & \\
Solver & \multicolumn{2}{c}{$\#$Timeouts}  & \multicolumn{2}{c|}{PAR1} & \multicolumn{2}{c}{$\#$Timeouts}  & \multicolumn{2}{c|}{PAR1} & Configurator\\
 & default & config. & default & config. & default & config. & default & config. & \\ 
\hline
\clasp & $86$ & $87$ & $80.79$ & $82.49$ & $\mathbf{87}$ & $93$ & $\mathbf{85.30}$ & $88.51$ & paramils-2\\
\lingeling & $93$ & $94$ & $90.40$ & $90.88$ & $101$ & $104$ & $96.94$ & $99.05$ & smac-disc-0\\
\cryptominisat & $89$ & $\mathbf{86}$ & $84.63$ & $85.40$ & $95$ & $\mathbf{89}$ & $90.04$ & $89.81$ & smac-disc-1\\
\riss & $90$ & $\mathbf{85}$ & $84.02$ & $81.95$ & $91$ & $88$ & $89.03$ & $\mathbf{85.72}$ & paramils-1\\
\sparrow & $92$ & $\mathbf{86}$ & $130.00$ & $\mathbf{83.70}$ & $98$ & $\mathbf{94}$ & $132.19$ & $\mathbf{90.93}$ & smac-2\\
\minisathack & $88$ & $\mathbf{83}$ & $82.15$ & $81.35$ & $91$ & $91$ & $85.44$ & $84.90$ & paramils-0\\
\yalsat & $223$ & $\mathbf{210}$ & $199.87$ & $\mathbf{188.63}$ & $218$ & $\mathbf{207}$ & $191.44$ & $\mathbf{183.74}$ & smac-0\\
\hline\hline
\end{tabular}
\caption{CSSC14: Track: \crafted; Benchmarks: \labs}
\end{table}

\begin{table}[h]
\footnotesize
\begin{tabular}{l | cccc | cccc | l}
\hline\hline
 & \multicolumn{4}{c|}{Training performance} & \multicolumn{4}{c|}{Test performance} & \\
Solver & \multicolumn{2}{c}{$\#$Timeouts}  & \multicolumn{2}{c|}{PAR1} & \multicolumn{2}{c}{$\#$Timeouts}  & \multicolumn{2}{c|}{PAR1} & Configurator\\
 & default & config. & default & config. & default & config. & default & config. & \\ 
\hline
\clasp & $132$ & $\mathbf{34}$ & $42.01$ & $\mathbf{23.08}$ & $43$ & $\mathbf{9}$ & $39.73$ & $\mathbf{20.31}$ & smac-2\\
\lingeling & $43$ & $\mathbf{24}$ & $28.09$ & $\mathbf{21.89}$ & $11$ & $\mathbf{5}$ & $27.49$ & $\mathbf{19.81}$ & smac-0\\
\cryptominisat & $115$ & $\mathbf{77}$ & $40.16$ & $\mathbf{36.37}$ & $43$ & $\mathbf{24}$ & $38.83$ & $\mathbf{34.79}$ & smac-disc-0\\
\riss & $133$ & $\mathbf{98}$ & $45.02$ & $\mathbf{40.51}$ & $43$ & $\mathbf{30}$ & $41.56$ & $\mathbf{36.55}$ & smac-1\\
\sparrow & $163$ & $\mathbf{123}$ & $125.86$ & $\mathbf{52.31}$ & $55$ & $\mathbf{42}$ & $115.02$ & $\mathbf{48.01}$ & smac-disc-1\\
\minisathack & $143$ & $\mathbf{142}$ & $44.76$ & $\mathbf{43.70}$ & $50$ & $50$ & $45.07$ & $\mathbf{44.47}$ & smac-disc-0\\
\yalsat & $590$ & $590$ & $173.26$ & $\mathbf{172.08}$ & $186$ & $186$ & $159.96$ & $\mathbf{159.44}$ & smac-disc-2\\
\hline\hline
\end{tabular}
\caption{CSSC14: Track: \crafted; Benchmarks: \gi}
\end{table}

\begin{table}[h]
\footnotesize
\begin{tabular}{l | cccc | cccc | l}
\hline\hline
 & \multicolumn{4}{c|}{Training performance} & \multicolumn{4}{c|}{Test performance} & \\
Solver & \multicolumn{2}{c}{$\#$Timeouts}  & \multicolumn{2}{c|}{PAR1} & \multicolumn{2}{c}{$\#$Timeouts}  & \multicolumn{2}{c|}{PAR1} & Configurator\\
 & default & config. & default & config. & default & config. & default & config. & \\ 
\hline
\clasp & $90$ & $\mathbf{0}$ & $71.13$ & $\mathbf{5.19}$ & $81$ & $\mathbf{0}$ & $81.84$ & $\mathbf{4.68}$ & smac-3\\
\lingeling & $3$ & $\mathbf{0}$ & $26.14$ & $\mathbf{17.57}$ & $3$ & $\mathbf{0}$ & $26.92$ & $\mathbf{17.38}$ & paramils-2\\
\cryptominisat & $4$ & $\mathbf{0}$ & $19.50$ & $\mathbf{8.83}$ & $2$ & $\mathbf{1}$ & $22.55$ & $\mathbf{9.62}$ & smac-disc-1\\
\riss & $3$ & $\mathbf{0}$ & $16.54$ & $\mathbf{6.77}$ & $2$ & $\mathbf{0}$ & $13.68$ & $\mathbf{7.31}$ & smac-disc-0\\
\sparrow & $10$ & $\mathbf{0}$ & $103.80$ & $\mathbf{7.79}$ & $3$ & $\mathbf{0}$ & $91.93$ & $\mathbf{8.52}$ & smac-disc-0\\
\minisathack & $0$ & $0$ & $10.98$ & $\mathbf{8.18}$ & $0$ & $0$ & $11.49$ & $\mathbf{8.38}$ & gga-disc-1\\
\yalsat & $484$ & $484$ & $300.00$ & $300.00$ & $351$ & $351$ & $300.00$ & $300.00$ & smac-disc-0\\
\hline\hline
\end{tabular}
\caption{CSSC14: Track: \crafted; Benchmarks: \queens}
\end{table}

%RANDOM SAT + UNSAT
\clearpage

\begin{table}[h]
\footnotesize
\begin{tabular}{l | cccc | cccc | l}
\hline\hline
 & \multicolumn{4}{c|}{Training performance} & \multicolumn{4}{c|}{Test performance} & \\
Solver & \multicolumn{2}{c}{$\#$Timeouts}  & \multicolumn{2}{c|}{PAR1} & \multicolumn{2}{c}{$\#$Timeouts}  & \multicolumn{2}{c|}{PAR1} & Configurator\\
 & default & config. & default & config. & default & config. & default & config. & \\ 
\hline
\clasp & $0$ & $0$ & $11.36$ & $\mathbf{4.11}$ & $0$ & $0$ & $7.91$ & $\mathbf{2.66}$ & smac-3\\
\dccsat & $0$ & $0$ & $81.07$ & $\mathbf{16.44}$ & $0$ & $0$ & $74.75$ & $\mathbf{15.01}$ & gga-1\\
\minisathack & $7$ & $\mathbf{0}$ & $35.36$ & $\mathbf{22.19}$ & $5$ & $\mathbf{1}$ & $30.77$ & $\mathbf{14.86}$ & paramils-1\\
\riss & $7$ & $\mathbf{2}$ & $38.34$ & $\mathbf{26.64}$ & $2$ & $2$ & $27.95$ & $\mathbf{20.42}$ & smac-disc-2\\
\sparrow & $24$ & $\mathbf{3}$ & $104.32$ & $\mathbf{28.89}$ & $8$ & $\mathbf{1}$ & $89.67$ & $\mathbf{20.99}$ & smac-2\\
\hline\hline
\end{tabular}
\caption{CSSC14: Track: \random; Benchmarks: \kthree}
\end{table}

\begin{table}[h]
\footnotesize
\begin{tabular}{l | cccc | cccc | l}
\hline\hline
 & \multicolumn{4}{c|}{Training performance} & \multicolumn{4}{c|}{Test performance} & \\
Solver & \multicolumn{2}{c}{$\#$Timeouts}  & \multicolumn{2}{c|}{PAR1} & \multicolumn{2}{c}{$\#$Timeouts}  & \multicolumn{2}{c|}{PAR1} & Configurator\\
 & default & config. & default & config. & default & config. & default & config. & \\ 
\hline
\clasp & $0$ & $0$ & $0.74$ & $\mathbf{0.30}$ & $0$ & $0$ & $0.74$ & $\mathbf{0.30}$ & paramils-3\\
\dccsat & $0$ & $0$ & $149.65$ & $\mathbf{29.64}$ & $1$ & $\mathbf{0}$ & $150.73$ & $\mathbf{29.90}$ & paramils-2\\
\minisathack & $0$ & $0$ & $1.86$ & $\mathbf{0.84}$ & $0$ & $0$ & $1.83$ & $\mathbf{0.81}$ & smac-disc-3\\
\riss & $0$ & $0$ & $2.55$ & $\mathbf{1.32}$ & $1$ & $\mathbf{0}$ & $3.72$ & $\mathbf{1.31}$ & paramils-2\\
\sparrow & $0$ & $0$ & $152.06$ & $\mathbf{1.44}$ & $0$ & $0$ & $149.46$ & $\mathbf{1.45}$ & paramils-3\\
\hline\hline
\end{tabular}
\caption{CSSC14: Track: \random; Benchmarks: \unif}
\end{table}

\begin{table}[h]
\footnotesize
\begin{tabular}{l | cccc | cccc | l}
\hline\hline
 & \multicolumn{4}{c|}{Training performance} & \multicolumn{4}{c|}{Test performance} & \\
Solver & \multicolumn{2}{c}{$\#$Timeouts}  & \multicolumn{2}{c|}{PAR1} & \multicolumn{2}{c}{$\#$Timeouts}  & \multicolumn{2}{c|}{PAR1} & Configurator\\
 & default & config. & default & config. & default & config. & default & config. & \\ 
\hline
\clasp & $41$ & $\mathbf{0}$ & $114.52$ & $\mathbf{35.83}$ & $18$ & $\mathbf{0}$ & $115.05$ & $\mathbf{35.03}$ & smac-2\\
\dccsat & $0$ & $0$ & $84.58$ & $\mathbf{19.35}$ & $1$ & $\mathbf{0}$ & $80.53$ & $\mathbf{18.94}$ & smac-1\\
\minisathack & $301$ & $\mathbf{171}$ & $236.85$ & $\mathbf{178.96}$ & $166$ & $\mathbf{99}$ & $246.70$ & $\mathbf{190.03}$ & paramils-3\\
\riss & $295$ & $\mathbf{221}$ & $233.84$ & $\mathbf{207.40}$ & $160$ & $\mathbf{113}$ & $241.02$ & $\mathbf{210.81}$ & smac-3\\
\sparrow & $253$ & $242$ & $\mathbf{162.00}$ & $213.78$ & $126$ & $126$ & $\mathbf{156.64}$ & $219.49$ & paramils-2\\
\hline\hline
\end{tabular}
\caption{CSSC14: Track: \random; Benchmarks: \threecnf}
\end{table}

% RANDOM SAT
\clearpage

\begin{table}[h]
\footnotesize
\begin{tabular}{l | cccc | cccc | l}
\hline\hline
& \multicolumn{4}{c|}{Training performance} & \multicolumn{4}{c|}{Test performance} & \\
Solver & \multicolumn{2}{c}{$\#$Timeouts}  & \multicolumn{2}{c|}{PAR1} & \multicolumn{2}{c}{$\#$Timeouts}  & \multicolumn{2}{c|}{PAR1} & Configurator\\
& default & config. & default & config. & default & config. & default & config. & \\
\hline
\probsat & $11$ & $\mathbf{2}$ & $19.42$ & $\mathbf{5.94}$ & $10$ & $\mathbf{4}$ & $24.22$ & $\mathbf{9.33}$ & smac-disc-0\\
\sparrow & $11$ & $\mathbf{3}$ & $18.54$ & $\mathbf{7.38}$ & $9$ & $\mathbf{5}$ & $18.61$ & $\mathbf{9.62}$ & smac-2\\
\csccsat & $2$ & $\mathbf{1}$ & $6.47$ & $5.76$ & $2$ & $2$ & $5.64$ & $6.01$ & smac-2\\
\yalsat & $9$ & $\mathbf{3}$ & $16.97$ & $\mathbf{12.72}$ & $\mathbf{6}$ & $7$ & $13.27$ & $14.22$ & paramils-2\\
\clasp & $250$ & $250$ & $300.00$ & $300.00$ & $250$ & $250$ & $300.00$ & $300.00$ & smac-disc-0\\
\minisathack & $250$ & $250$ & $300.00$ & $300.00$ & $250$ & $250$ & $300.00$ & $300.00$ & smac-disc-2\\
\hline\hline
\end{tabular}
\caption{CSSC14: Track: \randomsat; Benchmarks: \threesatonek}
\end{table}

\begin{table}[h]
\footnotesize
\begin{tabular}{l | cccc | cccc | l}
\hline\hline
 & \multicolumn{4}{c|}{Training performance} & \multicolumn{4}{c|}{Test performance} & \\
Solver & \multicolumn{2}{c}{$\#$Timeouts}  & \multicolumn{2}{c|}{PAR1} & \multicolumn{2}{c}{$\#$Timeouts}  & \multicolumn{2}{c|}{PAR1} & Configurator\\
 & default & config. & default & config. & default & config. & default & config. & \\
\hline
\probsat & $30$ & $\mathbf{2}$ & $93.53$ & $\mathbf{24.16}$ & $24$ & $\mathbf{0}$ & $78.10$ & $\mathbf{14.72}$ & smac-disc-2\\
\sparrow & $13$ & $\mathbf{1}$ & $32.80$ & $\mathbf{11.33}$ & $3$ & $3$ & $19.75$ & $\mathbf{11.04}$ & smac-disc-0\\
\csccsat & $9$ & $7$ & $25.30$ & $23.32$ & $\mathbf{3}$ & $6$ & $17.69$ & $20.11$ & gga-disc-1\\
\yalsat & $7$ & $\mathbf{4}$ & $27.82$ & $28.08$ & $5$ & $5$ & $24.49$ & $21.70$ & paramils-1\\
\clasp & $250$ & $\mathbf{249}$ & $300.00$ & $\mathbf{299.13}$ & $250$ & $250$ & $300.00$ & $300.00$ & smac-disc-0\\
\minisathack & $250$ & $250$ & $300.00$ & $300.00$ & $250$ & $250$ & $300.00$ & $300.00$ & smac-disc-0\\
\hline\hline
\end{tabular}
\caption{CSSC14: Track: \randomsat; Benchmarks: \sevensatninety}
\end{table}

\begin{table}[h]
\footnotesize
\begin{tabular}{l | cccc | cccc | l}
\hline\hline
 & \multicolumn{4}{c|}{Training performance} & \multicolumn{4}{c|}{Test performance} & \\
Solver & \multicolumn{2}{c}{$\#$Timeouts}  & \multicolumn{2}{c|}{PAR1} & \multicolumn{2}{c}{$\#$Timeouts}  & \multicolumn{2}{c|}{PAR1} & Configurator\\
 & default & config. & default & config. & default & config. & default & config. & \\
\hline
\probsat & $250$ & $\mathbf{0}$ & $300.00$ & $\mathbf{1.88}$ & $250$ & $\mathbf{0}$ & $300.00$ & $\mathbf{1.97}$ & smac-3\\
\sparrow & $250$ & $\mathbf{0}$ & $300.00$ & $\mathbf{6.57}$ & $250$ & $\mathbf{0}$ & $300.00$ & $\mathbf{6.23}$ & smac-disc-2\\
\csccsat & $0$ & $0$ & $7.08$ & $7.07$ & $0$ & $0$ & $\mathbf{6.77}$ & $6.80$ & paramils-1\\
\yalsat & $0$ & $0$ & $6.80$ & $\mathbf{4.44}$ & $0$ & $0$ & $4.89$ & $4.60$ & smac-disc-0\\
\clasp & $250$ & $250$ & $300.00$ & $300.00$ & $250$ & $250$ & $300.00$ & $300.00$ & smac-disc-0\\
\minisathack & $250$ & $250$ & $300.00$ & $300.00$ & $250$ & $250$ & $300.00$ & $300.00$ & smac-disc-0\\
\hline\hline
\end{tabular}
\caption{CSSC14: Track: \randomsat; Benchmarks: \fivesatfiveh}
\end{table}

%%%%%%%%%%%%%%%%%%%%%%%%%%%%%%%%%%%%%%%%%%%%%%%%%%%%%%%
%% Table of PAR10 values for CSSC13
%%%%%%%%%%%%%%%%%%%%%%%%%%%%%%%%%%%%%%%%%%%%%%%%%%%%%%%

\clearpage

\section{PAR$10$ Results for CSSC13}

\begin{table}[tp]
\sffamily\small\centering
\begin{tabular}{l | ccc}
\toprule[1.0pt]
 & \fivesatfiveh & \kthree & \unif \\
\midrule
\SolverFourtyThree & $3000 \to 3000$ & $94 \to 60$ & $1 \to \mathbf{1}$\\
\myrowcolour{}\clasp-cssc & $3000 \to 3000$ & $158 \to \mathbf{3}$ & $1 \to \mathbf{0}$\\
\forlnodrup & $3000 \to 3000$ & $491 \to \mathbf{118}$ & $4 \to \mathbf{1}$\\
\myrowcolour{}\gnoveltyGCa & $1997 \to \mathbf{77}$ & $1488 \to 1488$ & $3000 \to 3000$\\
\gnoveltyGCwa & $129 \to \mathbf{32}$ & $1488 \to 1488$ & $3000 \to 3000$\\
\myrowcolour{}\gnoveltyPCL & $3000 \to \mathbf{197}$ & $1488 \to 1488$ & $3000 \to 3000$\\
\lingeling & $3000 \to 3000$ & $120 \to \mathbf{8}$ & $2 \to \mathbf{1}$\\
\myrowcolour{}\rissg & $3000 \to 3000$ & $142 \to \mathbf{15}$ & $1 \to \mathbf{1}$\\
\rissgExt & $3000 \to 3000$ & $153 \to \mathbf{14}$ & $1 \to \mathbf{1}$\\
\myrowcolour{}\satj & $3000 \to 3000$ & $111 \to 85$ & $5 \to \mathbf{4}$\\
\simpsat & $3000 \to 3000$ & $73 \to 73$ & $3 \to \mathbf{3}$\\
\bottomrule[1.0pt]
\end{tabular}
\caption{PAR$10$ performance of default and configured solvers on each scenario of \random. 
The best PAR$10$ values are shown in bold faces where the performance difference 
is statistically significant 
(according to a permutation test with $100000$ permutations)
at $\alpha=0.05$.
}
\end{table}
\begin{table}[tp]
\sffamily\small\centering
\begin{tabular}{l | cccc}
\toprule[1.0pt]
 & \textit{BMC} & \circuit & \textit{IBM} & \textit{SWV} \\
\midrule
\SolverFourtyThree & $321 \to 321$ & $216 \to 217$ & $771 \to \mathbf{769}$ & $6 \to \mathbf{2}$\\
\myrowcolour{}\clasp-cssc & $667 \to \mathbf{436}$ & $278 \to \mathbf{181}$ & $712 \to \mathbf{710}$ & $0 \to \mathbf{0}$\\
\forlnodrup & $529 \to \mathbf{385}$ & $346 \to \mathbf{247}$ & $698 \to \mathbf{693}$ & $4 \to \mathbf{1}$\\
\myrowcolour{}\gnoveltyGCa & $2891 \to 2881$ & $\mathbf{2981} \to 3000$ & $2930 \to 2930$ & $2416 \to \mathbf{2159}$\\
\gnoveltyGCwa & $2891 \to \mathbf{2834}$ & $2991 \to \mathbf{2933}$ & $2930 \to 2930$ & $2425 \to \mathbf{2139}$\\
\myrowcolour{}\gnoveltyPCL & $2872 \to 2863$ & $3000 \to 3000$ & $2931 \to 2921$ & $2139 \to \mathbf{2137}$\\
\lingeling & $302 \to \mathbf{282}$ & $409 \to \mathbf{214}$ & $694 \to \mathbf{692}$ & $3 \to \mathbf{0}$\\
\myrowcolour{}\rissg & $332 \to 315$ & $217 \to 194$ & $700 \to \mathbf{690}$ & $1 \to \mathbf{0}$\\
\rissgExt & $332 \to \mathbf{201}$ & $227 \to \mathbf{174}$ & $700 \to \mathbf{470}$ & $1 \to \mathbf{0}$\\
\myrowcolour{}\satj & $725 \to 726$ & $381 \to \mathbf{320}$ & $778 \to \mathbf{767}$ & $16 \to \mathbf{3}$\\
\simpsat & $411 \to 383$ & $280 \to \mathbf{260}$ & $705 \to 696$ & $5 \to 5$\\
\bottomrule[1.0pt]
\end{tabular}
\caption{PAR$10$ performance of default and configured solvers on each scenario of \indu. 
The best PAR$10$ values are shown in bold faces where the performance difference 
is statistically significant 
(according to a permutation test with $100000$ permutations)
at $\alpha=0.05$.
}
\end{table}
\begin{table}[tp]
\sffamily\small\centering
\begin{tabular}{l | cc}
\toprule[1.0pt]
 & \gi & \labs \\
\midrule
\SolverFourtyThree & $570 \to \mathbf{558}$ & $780 \to 755$\\
\myrowcolour{}\clasp-cssc & $362 \to \mathbf{65}$ & $837 \to \mathbf{779}$\\
\forlnodrup & $348 \to \mathbf{77}$ & $822 \to 787$\\
\myrowcolour{}\gnoveltyGCa & $1565 \to \mathbf{1540}$ & $2054 \to \mathbf{1485}$\\
\gnoveltyGCwa & $1541 \to \mathbf{1540}$ & $1669 \to \mathbf{1329}$\\
\myrowcolour{}\gnoveltyPCL & $1535 \to 1526$ & $1707 \to \mathbf{1571}$\\
\lingeling & $370 \to \mathbf{95}$ & $907 \to \mathbf{838}$\\
\myrowcolour{}\rissg & $439 \to \mathbf{362}$ & $838 \to \mathbf{770}$\\
\rissgExt & $431 \to \mathbf{18}$ & $845 \to \mathbf{367}$\\
\myrowcolour{}\satj & $534 \to \mathbf{491}$ & $951 \to \mathbf{897}$\\
\simpsat & $366 \to 366$ & $923 \to 923$\\
\bottomrule[1.0pt]
\end{tabular}
\caption{PAR$10$ performance of default and configured solvers on each scenario of \crafted. 
The best PAR$10$ values are shown in bold faces where the performance difference 
is statistically significant 
(according to a permutation test with $100000$ permutations)
at $\alpha=0.05$.
}
\end{table}

\section{PAR$10$ Results for CSSC14}

\begin{table}[tp]
\sffamily\small\centering
\begin{tabular}{l | ccc}
\toprule[1.0pt]
 & \threecnf & \kthree & \unif \\
\midrule
\dccsat & $91 \to \mathbf{19}$ & $75 \to \mathbf{15}$ & $162 \to \mathbf{30}$\\
\myrowcolour{}\riss & $1969 \to \mathbf{1431}$ & $50 \to 42$ & $15 \to \mathbf{1}$\\
\sparrow & $1517 \to 1580$ & $176 \to \mathbf{32}$ & $149 \to \mathbf{1}$\\
\myrowcolour{}\clasp & $309 \to \mathbf{35}$ & $8 \to \mathbf{3}$ & $1 \to \mathbf{0}$\\
\minisathack & $2040 \to \mathbf{1259}$ & $85 \to \mathbf{26}$ & $2 \to \mathbf{1}$\\
\bottomrule[1.0pt]
\end{tabular}
\caption{PAR$10$ performance of default and configured solvers on each scenario of \random. 
The best PAR$10$ values are shown in bold faces where the performance difference 
is statistically significant 
(according to a permutation test with $100$ permutations)
at $\alpha=0.05$.
}
\end{table}
\begin{table}[tp]
\sffamily\small\centering
\begin{tabular}{l | ccc}
\toprule[1.0pt]
 & \threesatonek & \fivesatfiveh & \sevensatninety \\
\midrule
\csccsat & $27 \to 28$ & $\mathbf{7} \to 7$ & $\mathbf{50} \to 85$\\
\myrowcolour{}\sparrow & $116 \to \mathbf{64}$ & $3000 \to \mathbf{6}$ & $52 \to 43$\\
\yalsat & $78 \to 90$ & $5 \to 5$ & $78 \to 76$\\
\myrowcolour{}\clasp & $3000 \to 3000$ & $3000 \to 3000$ & $3000 \to 3000$\\
\minisathack & $3000 \to 3000$ & $3000 \to 3000$ & $3000 \to 3000$\\
\myrowcolour{}\probsat & $132 \to \mathbf{53}$ & $3000 \to \mathbf{2}$ & $337 \to \mathbf{15}$\\
\bottomrule[1.0pt]
\end{tabular}
\caption{PAR$10$ performance of default and configured solvers on each scenario of \randomsat. 
The best PAR$10$ values are shown in bold faces where the performance difference 
is statistically significant 
(according to a permutation test with $100$ permutations)
at $\alpha=0.05$.
}
\end{table}
\begin{table}[tp]
\sffamily\small\centering
\begin{tabular}{l | ccc}
\toprule[1.0pt]
 & \bmc & \circuit & \hw \\
\midrule
\riss & $421 \to \mathbf{285}$ & $218 \to 234$ & $721 \to \mathbf{721}$\\
\myrowcolour{}\sparrow & $744 \to \mathbf{383}$ & $433 \to \mathbf{227}$ & $798 \to \mathbf{724}$\\
\clasp & $451 \to \mathbf{316}$ & $194 \to \mathbf{135}$ & $710 \to 710$\\
\myrowcolour{}\cryptominisat & $428 \to 405$ & $328 \to \mathbf{215}$ & $703 \to 695$\\
\lingeling & $222 \to \mathbf{221}$ & $316 \to \mathbf{193}$ & $697 \to \mathbf{694}$\\
\myrowcolour{}\minisathack & $233 \to 232$ & $226 \to 204$ & $699 \to \mathbf{698}$\\
\bottomrule[1.0pt]
\end{tabular}
\caption{PAR$10$ performance of default and configured solvers on each scenario of \indu. 
The best PAR$10$ values are shown in bold faces where the performance difference 
is statistically significant 
(according to a permutation test with $100$ permutations)
at $\alpha=0.05$.
}
\end{table}
\begin{table}[tp]
\sffamily\small\centering
\begin{tabular}{l | ccc}
\toprule[1.0pt]
 & \gi & \labs & \queens \\
\midrule
\riss & $372 \to \mathbf{267}$ & $789 \to 763$ & $29 \to \mathbf{7}$\\
\myrowcolour{}\sparrow & $538 \to \mathbf{371}$ & $886 \to \mathbf{814}$ & $115 \to \mathbf{9}$\\
\yalsat & $1591 \to \mathbf{1590}$ & $1868 \to \mathbf{1776}$ & $3000 \to 3000$\\
\myrowcolour{}\clasp & $370 \to \mathbf{90}$ & $755 \to 804$ & $705 \to \mathbf{5}$\\
\cryptominisat & $370 \to \mathbf{219}$ & $821 \to 774$ & $38 \to \mathbf{17}$\\
\myrowcolour{}\lingeling & $112 \to \mathbf{58}$ & $874 \to 899$ & $50 \to \mathbf{17}$\\
\minisathack & $430 \to \mathbf{429}$ & $785 \to 785$ & $11 \to \mathbf{8}$\\
\bottomrule[1.0pt]
\end{tabular}
\caption{PAR$10$ performance of default and configured solvers on each scenario of \crafted. 
The best PAR$10$ values are shown in bold faces where the performance difference 
is statistically significant 
(according to a permutation test with $100$ permutations)
at $\alpha=0.05$.
}
\end{table}

\begin{table}[th]
\sffamily\small\centering
\setlength\tabcolsep{0.3em}
\begin{tabular}{l | ccccc | ccccc}
\toprule[1pt]
 & \multicolumn{5}{c|}{Training} & \multicolumn{5}{c}{Test}\\
 & \smac{}-d & \smac{}-c & \pils{} & \gga{}-d & \gga{}-c & \smac{}-d & \smac{}-c & \pils{} & \gga{}-d & \gga{}-c  \\
\midrule
\csccsat & $1.8$ & $1.8$ & $1.8$ & $0.5$ & $0.7$ & $0.6$ & $0.6$ & $0.6$ & $1.0$ & $0.7$\\
\dccsat & $4.7$ & $4.7$ & $4.7$ & $1.5$ & $4.7$ & $5.0$ & $5.0$ & $5.1$ & $1.5$ & $5.0$\\
\riss & $2.7$ & $2.7$ & $2.1$ & $0.5$ & $0.9$ & $2.2$ & $3.0$ & $2.3$ & $0.5$ & $1.1$\\
\sparrow & $11.9$ & $14.0$ & $7.5$ & $-$ & $-$ & $9.1$ & $9.6$ & $5.4$ & $-$ & $-$\\
\yalsat & $2.1$ & $1.1$ & $1.3$ & $0.2$ & $0.3$ & $1.4$ & $2.5$ & $0.8$ & $0.1$ & $0.6$\\
\clasp & $4.3$ & $3.2$ & $2.6$ & $-$ & $-$ & $2.8$ & $3.7$ & $2.3$ & $-$ & $-$\\
\cryptominisat & $2.7$ & $2.5$ & $2.1$ & $1.7$ & $2.1$ & $3.4$ & $2.7$ & $2.5$ & $2.3$ & $2.6$\\
\lingeling & $1.6$ & $1.5$ & $1.7$ & $-$ & $0.1$ & $1.4$ & $1.9$ & $1.4$ & $-$ & $0.1$\\
\minisathack & $1.9$ & $2.0$ & $2.0$ & $1.0$ & $1.2$ & $1.8$ & $1.7$ & $1.7$ & $1.3$ & $1.1$\\
\probsat & $95.8$ & $80.5$ & $86.9$ & $-$ & $-$ & $83.8$ & $55.9$ & $81.3$ & $-$ & $-$\\
\bottomrule[1pt]
\end{tabular}
\caption{CSSC'14: Geometric mean of speedups for each solver configured by different configurators}
\end{table}
